# Supplementary material for: ACMo: Angle-Calibrated Moment Methods for Stochastic Optimization
Source: arXiv:2006.07065 source file (2020-06-12)
Supplement: Supplementary file 1 [file 000_theorem_4_1.tex]

\begin{proof}
With Assumption~4.1 and Lemma~\ref{lem:subsequence_construction}, for the sequence $\{\vtheta_t^\prime\}$, we have
\begin{equation}
    \label{eq:thm_4_1_init}
    \begin{split}
        \mathbb{E}\left[f(\vtheta_{t+1}^\prime) - f(\vtheta_t^\prime)\right] \le \mathbb{E}\left[\nabla f^T(\vtheta_t^\prime)\left(\vtheta_{t+1}^\prime- \vtheta_t^\prime\right)+\frac{L}{2}\left\|\vtheta_{t+1}^\prime - \vtheta_t^\prime\right\|\right].
    \end{split}
\end{equation}
We obtain the telescoping sum as follows
\begin{equation}
    \label{eq:thm_4_1_tele_sum}
    \begin{split}
        \mathbb{E}\left[f(\vtheta_{t+1}^\prime - \vtheta_1^\prime)\right]\le & \mathbb{E}\left[\sum_{i=1}^t\left(\nabla f^T(\vtheta_i^\prime)\left(\vtheta_{i+1}^\prime-\vtheta_i^\prime\right)+\frac{L}{2}\left\|\vtheta_{i+1}^\prime-\vtheta_i^\prime\right\|\right)\right]\\
        \mathop{\le}^{\mathcircled1}& \underbrace{\mathbb{E}\left[\sum_{i=1}^t \nabla f^T(\vtheta_i^\prime)\left[\frac{-\alpha_i}{1-\frac{\hat{\beta}_i}{5}}\right]\rvg_i\right]}_{T_1} + \underbrace{\mathbb{E}\left[\sum_{i=1}^t \frac{L}{2}\left\|\vtheta_{i+1}^\prime - \vtheta_{i}^\prime\right\|^2\right]}_{T_2}\\
        &+\underbrace{\mathbb{E}\left[\sum_{i=2}^t \nabla f^T(\vtheta_i^\prime)\left[\frac{-\alpha_i}{1-\frac{\hat{\beta}_i}{5}}\left(1-\frac{\alpha_{i-1}}{5\alpha_{i}}\right)\right]\hat{\beta}_i\hat{\rvm}_{i-1}\right]}_{T_3}\\
        &+\underbrace{\mathbb{E}\left[\sum_{i=1}^t \nabla f^T(\vtheta_i^\prime)\left[\frac{\hat{\beta}_i}{5-\hat{\beta}_i}-\frac{\hat{\beta}_{i+1}}{5-\hat{\beta}_{i+1}}\alpha_i\hat{\rvm}_i\right]\right]}_{T_4},
    \end{split}
\end{equation}
where $\mathcircled1$ establishes because of the Lemma~\ref{lem:subsequence_construction}.
\end{proof}
