# Supplementary material for: ACMo: Angle-Calibrated Moment Methods for Stochastic Optimization
Source: arXiv:2006.07065 source file (2020-06-12)
Supplement: Supplementary file 2 [file 002_lemmas_for_theorem_4_1.tex]

\begin{proof}
    By introducing the sequence $\{\vtheta_t\}$, we have
    \begin{equation*}
        \begin{split}
            & \mathbb{E}\left[\nabla f^T(\vtheta_i^\prime)\left[\frac{-\alpha_i}{1-\frac{\hat{\beta}_i}{5}}\left(1-\frac{\alpha_{i-1}}{5\alpha_{i}}\right)\right]\hat{\beta}_i\hat{\rvm}_{i-1}\right]\\
            =& \underbrace{\mathbb{E}\left[\left(\nabla f(\vtheta_i^\prime) - \nabla f(\vtheta_i)\right)^T\left[\frac{-\alpha_i}{1-\frac{\hat{\beta}_i}{5}}\left(1-\frac{\alpha_{i-1}}{5\alpha_{i}}\right)\hat{\beta}_i\hat{\rvm}_{i-1}\right]\right]}_{T_{3.1}}+ \underbrace{\mathbb{E}\left[\nabla f^T(\vtheta_i)\left[\frac{-\alpha_i}{1-\frac{\hat{\beta}_i}{5}}\left(1-\frac{\alpha_{i-1}}{5\alpha_{i}}\right)\hat{\beta}_i\hat{\rvm}_{i-1}\right]\right]}_{T_{3.2}}
        \end{split}
    \end{equation*}

    Before bounding $T_{3.1}$, we request $1\le \frac{\alpha_{i-1}}{\alpha_i}\le 2$ for any $i$, and obtain
    \begin{equation*}
        \frac{3}{5}\le 1-\frac{\alpha_{i-1}}{5\alpha_i}\le \frac{4}{5}.
    \end{equation*}
    $T_{3.1}$ satisfies the following inequalities.
    \begin{equation}
        \label{eq:thm_4_T_3_1_bound}
        \begin{split}
            T_{3.1} =& \mathbb{E}\left[\left(\nabla f(\vtheta_i^\prime) - \nabla f(\vtheta_i)\right)^T\left[\frac{-\alpha_i}{1-\frac{\hat{\beta}_i}{5}}\left(1-\frac{\alpha_{i-1}}{5\alpha_{i}}\right)\cdot\frac{\left\|\rvg_i\right\|}{\left\|\hat{\rvm}_{i-1}\right\|+\delta_i}\cdot \beta_i\hat{\rvm}_{i-1}\right]\right]\\
            \le & \mathbb{E}\left[\left\|\nabla f(\vtheta_i^\prime) - \nabla f(\vtheta_i)\right\|\cdot\left(\frac{\alpha_i}{1-\frac{\hat{\beta}_i}{5}}\right)\cdot\left(1-\frac{\alpha_{i-1}}{5\alpha_i}\right)\cdot\beta_i\left\|\rvg_i\right\|\right]\\
            \le & \mathbb{E}\left[L\left\|\vtheta_i^\prime - \vtheta_i\right\|\cdot\left(\frac{\alpha_i}{1-\frac{\hat{\beta}_i}{5}}\right)\cdot\left(1-\frac{\alpha_{i-1}}{5\alpha_i}\right)\cdot\beta_i\left\|\rvg_i\right\|\right]\\
            = & \mathbb{E}\left[L\left(\frac{\hat{\beta}_i}{5-\hat{\beta}_i}\right)\alpha_{i-1}\left\|\hat{\rvm}_{i-1}\right\|\cdot\left(\frac{\alpha_i}{1-\frac{\hat{\beta}_i}{5}}\right)\cdot\left(1-\frac{\alpha_{i-1}}{5\alpha_i}\right)\cdot\beta_i\left\|\rvg_i\right\|\right]\\
            = &\mathbb{E}\left[\frac{L\alpha_{i-1}}{5-\hat{\beta}_i}\cdot\beta_i\cdot\frac{\left\|\rvg_i\right\|}{\left\|\hat{\rvm}_{i-1}\right\|+\delta_i}\left\|\hat{\rvm}_{i-1}\right\|\cdot\frac{\alpha_i}{1-\frac{\hat{\beta}_i}{5}}\cdot\frac{4\beta_i}{5}\left\|\rvg_i\right\|\right]\\
            \le & \mathbb{E}\left[\frac{L\alpha_{i-1}}{5-\hat{\beta}_i}\cdot\frac{\alpha_i}{1-\frac{\hat{\beta}_i}{5}}\cdot\frac{4\beta_i^2}{5}\left\|\rvg_i\right\|^2\right] \mathop{\le}^{\mathcircled1} \mathbb{E}\left[\frac{\alpha_i}{1-\frac{\hat{\beta}_i}{5}}\cdot \frac{8\beta_i^2}{25}\left\|\rvg_i\right\|^2\right]\\
            =& \mathbb{E}\left[\frac{\alpha_i}{1-\frac{\hat{\beta}_i}{5}}\cdot \frac{8\beta_i^2}{25}\left\|\rvg_i-\nabla f(\vtheta_i) + \nabla f(\vtheta_i)\right\|^2\right]\\
            \le & \mathbb{E}\left[\frac{\alpha_i}{1-\frac{\hat{\beta}_i}{5}}\cdot \frac{4\beta_i^2}{25}\left\|\rvg_i-\nabla f(\vtheta_i)\right\|^2\right] + \mathbb{E}\left[\frac{\alpha_i}{1-\frac{\hat{\beta}_i}{5}}\cdot \frac{4\beta_i^2}{25}\left\|\nabla f(\vtheta_i)\right\|^2\right]\\
            \le& \frac{\alpha_i}{1-\frac{\hat{\beta}_i}{5}}\cdot \frac{4\beta_i^2}{25}\cdot\sigma^2+ \mathbb{E}\left[\frac{\alpha_i}{1-\frac{\hat{\beta}_i}{5}}\cdot \frac{4\beta_i^2}{25}\left\|\nabla f(\vtheta_i)\right\|^2\right],
        \end{split}
    \end{equation}
    where $\mathcircled1$ is satisfied because we can choose the hyper-parameters as Corollary~\ref{cor:iter_con_bound}, and obtain $L\alpha_{i-1}\le 1$ and $\hat{\beta}_i \le \frac{5}{2}$.
    
    Then, for $T_{3.2}$, we have 
    \begin{equation}
        \label{eq:thm_4_T_3_2_bound}
        \begin{split}
            T_{3.2} =& \mathbb{E}\left[\nabla f^T(\vtheta_i)\left[\frac{-\alpha_i}{1-\frac{\hat{\beta}_i}{5}}\cdot\left(1-\frac{\alpha_{i-1}}{5\alpha_i}\right)\cdot\frac{\left\|\rvg_i\right\|}{\left\|\hat{\rvm}_{i-1}\right\|+\delta_i}\cdot\beta_i\hat{\rvm}_{i-1}\right]\right]\\
            \le & \mathbb{E}\left[\frac{\alpha_i}{1-\frac{\hat{\beta}_i}{5}}\cdot \left[\frac{1}{8}\left\|\nabla f(\vtheta_i)\right\|^2 + 2\left(1-\frac{\alpha_{i-1}}{5\alpha_i}\right)^2\left(\frac{\left\|\rvg_i\right\|}{\left\|\hat{\rvm}_{i-1}\right\|+\delta_i}\right)^2\beta_i^2 \left\|\hat{\rvm}_{i-1}\right\|^2\right]\right]\\
            \le & \mathbb{E}\left[\frac{\alpha_i}{1-\frac{\hat{\beta}_i}{5}}\cdot \frac{1}{8}\left\|\nabla f(\vtheta_i)\right\|^2\right] + \mathbb{E}\left[\frac{\alpha_i}{1-\frac{\hat{\beta}_i}{5}}\cdot \frac{32}{25}\beta_i^2\left\|\rvg_i\right\|^2\right]\\
            = & \mathbb{E}\left[\frac{\alpha_i}{1-\frac{\hat{\beta}_i}{5}}\cdot \frac{1}{8}\left\|\nabla f(\vtheta_i)\right\|^2\right] + \mathbb{E}\left[\frac{\alpha_i}{1-\frac{\hat{\beta}_i}{5}}\cdot \frac{32}{25}\beta_i^2\left\|\rvg_i-\nabla f(\vtheta_i)+\nabla f(\vtheta_i)\right\|^2\right]\\
            \le & \mathbb{E}\left[\frac{\alpha_i}{1-\frac{\hat{\beta}_i}{5}}\cdot \frac{1}{8}\left\|\nabla f(\vtheta_i)\right\|^2\right] + \mathbb{E}\left[\frac{\alpha_i}{1-\frac{\hat{\beta}_i}{5}}\cdot \frac{16}{25}\beta_i^2\left\|\rvg_i-\nabla f(\vtheta_i)\right\|^2\right] +\\
            & \mathbb{E}\left[\frac{\alpha_i}{1-\frac{\hat{\beta}_i}{5}}\cdot \frac{16}{25}\beta_i^2\left\|\nabla f(\vtheta_i)\right\|^2\right]\\
            \le & \mathbb{E}\left[\frac{\alpha_i}{1-\frac{\hat{\beta}_i}{5}}\cdot \frac{1}{8}\left\|\nabla f(\vtheta_i)\right\|^2\right] + \mathbb{E}\left[\frac{\alpha_i}{1-\frac{\hat{\beta}_i}{5}}\cdot \frac{16}{25}\beta_i^2\left\|\nabla f(\vtheta_i)\right\|^2\right] + \frac{\alpha_i}{1-\frac{\hat{\beta}_i}{5}}\cdot \frac{16}{25}\beta_i^2\sigma^2
        \end{split}
    \end{equation}
    %where $\mathcircled1$ and $\mathcircled2$ establish because of the Assumption~4.1 and the definition of $\hat{\beta}_i$.
\end{proof}
